# Supplementary material for: On the Feasibility of Using MultiModal LLMs to Execute AR Social Engineering Attacks
Source: arXiv:2504.13209 source file (2025-04-16)
Supplement: Supplementary file 1 [file appendix.tex]

\appendix

\section{Appendices}

\subsection{ReInteract SE Agent Algorithm}
\label{sec:appendix_agent_algorithm}

\begin{algorithm}[h]
\small
    \caption{ReInteract SE Agent} \label{algorithm:agent}
    \begin{algorithmic}[1]
        \REQUIRE Preset SE Strategy Templates $T$ from the attacker, target social profile $p$ from the multimodal LLM.
        \ENSURE conversation $C$

        \Comment Select SE strategy for target
        \STATE $t \gets CheckSEStrategies(T, p)$

        %\Comment Create thought generator $G()$
        %\STATE $G() \gets BuildThought(||p||, D)$

        %\Comment Create action function $Act()$
        %\STATE $Act() \gets BuildActionRAG(||p||, D)$

        %\Comment Decompose NL policy $p_{NL}$
        %\STATE $E \gets Decompose(p_{NL}, G(), Act())$

        \STATE $C \gets \emptyset$

        \Comment Reasoning and Interaction Cycle
        \FORALL{$s \in t$}
            %\Comment
            \STATE $c_s \gets GenConv(C, p, s)$

            \STATE $r_s \gets SEInteract(c_s)$
            
            \STATE $C \gets C + c_s + r_s$
        \ENDFOR
        \STATE return $C$
    \end{algorithmic}
\end{algorithm}

\subsection{Age Distribution}
\label{sec:appendix_age_distribution}

\begin{figure}[h]
\centering
\includegraphics[width=0.95\linewidth]{drawings/age distribution.png}
\caption{Participant Age Distribution Curve}
\label{fig:dataset_age}
\end{figure}
